# Supplementary material for: Universal quantum control of two-electron spin quantum bits using dynamic nuclear polarization
Source: arXiv:1009.5343 ancillary file (2010-09-27)
Supplement: Supplementary file 1 [file supplement.pdf]

# Universal quantum control of two-electron spin quantum bits using dynamic nuclear polarization - Supplementary Material

Sandra Foletti,[1] Hendrik Bluhm,[1] Diana Mahalu,[2] Vladimir Umansky,[2] and Amir Yacoby[1]

[1]*Department of Physics, Harvard University, Cambridge, MA 02138, USA*
[2]*Braun Center for Submicron Research, Department of Condensed Matter Physics, Weizmann Institute of Science, Rehovot 76100, Israel*

In the first three sections of this document, we provide further technical details on our experiment. This includes details on our quantum point contact (QPC) operating point and additional explanations of the pump and measurement pulse cycles. We also give a more detailed explanation of the analysis and the model used to fit the data in Fig. 4. In the remaining three sections, we discuss empirical observations that are not fundamental to the reported work, but might be important for understanding the mechanism leading to a strongly inhomogeneous polarization in the two dots.

## I. QPC OPERATION AND GATE LEVER ARM

The quantum point contact (QPC) was operated at a 2 nA rms ac bias current and a conductance of approximately 0.4 $G_0$, where $G_0 = 2e^2/h$ is the conductance quantum. The signal change across the (1,1)-(0,2) charge transition was typically 2 to 4 $\mu$V (corresponding to a conductance change of 2-4 %). We note that since the ground state is a singlet ($S$), the signal corresponding to a singlet ($p(S) = 1$) is well known, whereas that corresponding to a triplet ($p(S) = 0$) is affected by the inelastic triplet decay rate during the measurement stage [1]. This decay rate varies with dot tuning, $B_{ext}$ and apparently polarization, and is different for $T_0$ and $T_+$. Because of these uncertainties in the signal conversion, we normalize the QPC signal by the size of the DC charge transition and denote the result by $P_S$.

In the measurement pulse illustrated in Fig. 1e, the system is reset in $S$(0,2) at point **M**, then the gates are moved to point **S** by a voltage change of 7 mV on both GR and GL. After a mixing time $\tau_S$ they are set back to point **M** for the rest of the 12 $\mu s$ total pulse period. In the $S$ and $T_+$-pump cycles (see Fig. 1f, g), GL and GR are ramped over 0.5 mV across the $S$-$T_+$ transition in 50 ns (100 ns) with 4 MHz (1.1 MHz) repetition rate. Changes in gate voltage can be converted to energy shifts with a conversion factor ≈0.1 eV/V extracted from transport measurements through the double dot at finite bias (transport measurements are shown in the upper panels in Supplementary Fig. 4).

## II. MODEL AND FIT PROCEDURES FOR TOMOGRAPHY DATA

While the contrast in the measurement triangle should be a direct measure of the singlet return probability, we find empirically that it varies with polarization, position of the measurement point **M**, and pulse shape, as discussed in section IV. In the tomography measurement (Fig. 4) we account for the imperfect pulse shape errors by monitoring the QPC signal from a reference pulse without any excursion to (1,1) and the $\tau_{rot} = 0$ pulses to convert the measured signal to probabilities. Both the reference pulse and the $\tau_{rot} = 0$ X-pulse should produce a singlet-like signal. However, because of direct coupling of the pulses to the QPC, the two pulses result in a slightly different QPC conductance. This correction is approximately proportional to the time spent in (1,1) and thus mostly due to the long ramps for preparation and X-readout. For the Y and Z-pulses, which contain only one ramp each, we have used the average of the signals from the reference pulse (no ramp) and the $\tau_{rot} = 0$ X-pulse (two ramps) to determine $p(|S\rangle) = p(|Z\rangle) = 1$ and $p(|S\rangle + i|T_0\rangle) = p(|Y\rangle) = 1$, while $p(|Z\rangle) = 1/2$ and $p(|Y\rangle) = 1/2$ are determined from the average of the $\tau_{rot} = 0$ Y and Z-pulse signals. For the X-pulse, only the $p(|\uparrow\downarrow\rangle) = p(|X\rangle) = 1$ signal can be determined reliably. We have thus adjusted the remaining scaling factor manually such that the amplitude of the Y-signal obtained from the fits as described below matches the data.

To fit the tomography data, we have numerically solved the Schrödinger equation for the Hamiltonian $H = J(t)/2\sigma_z + g\mu_B \Delta B^z_{nuc}/2\sigma_x$, with a time dependence of $J$ reflecting the finite rise time of the pulses. We have parametrized $J(\varepsilon)$ by a phenomenological exponential dependence $J(\varepsilon) \propto e^{\varepsilon/\epsilon}$ that approximates our measurements of the frequency of exchange oscillations (cf. [2,3]) as a function of $\varepsilon$. The time dependence of $\varepsilon$ was modeled as $\varepsilon(t) - \varepsilon(t = 0) \propto 1 - \alpha e^{-t/\tau_1} + (1 - \alpha)e^{-t/\tau_2}$. The time dependence of $\varepsilon$ and $J$ obtained from the fits is shown in Supplementary Fig. 1. The model was chosen such that it can produce a pulse shape with an initial fast rise followed by a slow decay. This behavior is expected because of the frequency dependent attenuation of the coaxial cables (Supplementary Fig. 1b) and other bandwidth limitations and can also be observed in exchange pulses with $\Delta B^z_{nuc} \ll J$. For comparison, the specified 10 to 90 % rise time of our pulse generator is 1.5 ns.

When switching on $J$ at the end of the preparation ramp, the fast part of the pulse is in a region where $J(\epsilon) \ll \Delta B^z_{nuc}$, so that $J$ increases significantly only in the slow phase of the pulse, leading to a slow rise of $J(t)$. When switching off $J$ or returning to (0,2), $J$ varies strongly in the fast part of the pulse, so that an infinitely sharp rise is a good approximation. We have

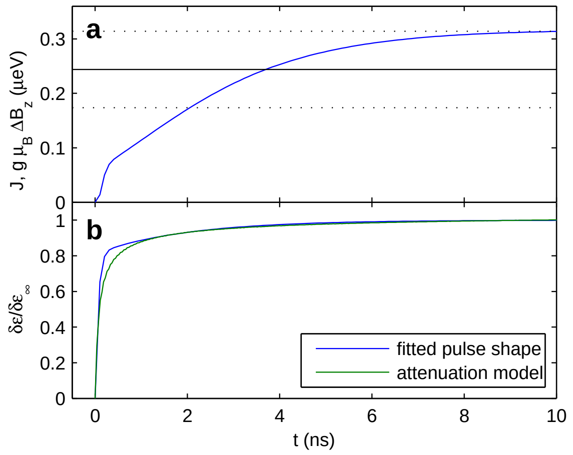


Supplementary Fig. 1: **Pulse shapes extracted from fits of the tomography data. a,** Time dependence of $J$ according to the fit model described in the text (blue line). The black line shows $\overline{\Delta B^z_{nuc}}$, the mean of $\Delta B^z_{nuc}$, and the dashed lines indicate the rms fluctuation amplitude, $\delta\Delta B^z_{nuc}$. **b,** Pulse shape corresponding to $J(t)$ from **a,** (blue line). The sharp kink is an artifact of the pulse parametrization. The green line shows the pulse expected from a step function transmitted through a lossy coax cable, with a time constant obtained by comparing the same model to the measured pulse shape on a similar experimental setup.

thus only considered the effect of a finite rise time when switching on $J$. To account for fluctuations in $\Delta B^z_{nuc}$, we have taken a weighted average of simulation results for a range of $\Delta B^z_{nuc}$ with Gaussian weights.

The data from the X and Z-pulses (Fig. 4b) were fitted simultaneously with the following fit parameters: $\alpha = 0.19$, $\tau_1 = 2.0$ ns, $\tau_2 = 0.064$ ns, $\epsilon = 0.44$ mV (normalized as change in gate voltages, i.e. $\sqrt{\Delta V_{GL}^2 + \Delta V_{GR}^2}$), $J_X = 0.32$ $\mu$eV, $J_Z = 0.45$ $\mu$eV, $\overline{\Delta B^z_{nuc}} = 10.5$ mT, $\delta\Delta B^z_{nuc} = 4.3$ mT. $\overline{\Delta B^z_{nuc}}$ and $\delta\Delta B^z_{nuc}$ denote the mean and standard deviation of the $\Delta B^z_{nuc}$ distribution and $J_X$ and $J_Z$ the asymptotic value of $J$ for the X and Z-pulse. Ideally, one could set $J_X = J_Z$, however in our data, different offsets to the pulses due to the DC blocking effect of our bias-T's (used to add the high bandwidth pulses to the DC gate voltages) lead to a $\approx 25\%$ difference. All other parameters were the same for both the X and the Z-fit. The model curve shown for Y was computed with the same parameter values and $J_Y = J_Z$. This is reasonable because the overall pulse shape of the Y-pulse is more similar to the one of the Z-pulse than the one of the X-pulse (see Fig. 4a). In the Bloch sphere representation of the model in Fig. 4d, the $J_Z$ value was used for all three coordinates.

## III. $S$-$T_+$ TRANSITION MEASUREMENT AND CALIBRATION

To probe the position of the $S$-$T_+$ transition, we have used a pulse as reported in Refs.[2,4]. It is similar to the $S$-pumping cycle, with the ramping through the $S$-$T_+$ transition replaced by a jump to and a wait time at the degeneracy point (typically 100 ns). In addition, it is extended with a measurement stage at point **M**, resulting in a total pulse period of 12 $\mu$s. Sweeping the DC value of GL and GR while running this pulse results in line scans as shown in Fig. 3c. When the $S$ and $T_+$ states are degenerate, transitions from the prepared $S$ to the $T_+$ state are allowed and cause a dip in $P_S$. For the data in Fig. 3, this measurement has been interleaved with the gradient-probing pulse at a fixed point, each running for 2 s with pumping in between. Thus, any polarization effect of either pulse will affect both measurements equally because the nuclear relaxation time is much longer than 2 s. To calibrate the shift in the $S$-$T_+$ transition, we have taken line scans along $\varepsilon$ as a function of external field $B_{ext}$ (Supplementary Fig. 2) and analyzed them in the same way as the measurement in Fig. 3a. We have fitted the field dependence of the position of the dip in $P_S$ with a polynomial. This allows to convert the shift in the $S$-$T_+$ transition in response to polarization to a change in field, which can be identified with $B^z_{nuc}$ if $\Delta B^z_{nuc} \ll B_{ext}$.

The analysis may be subject to various systematic errors. An imperfect alignment of the sample with the external magnetic field may lead to orbital effects contributing to the calibration of the position of the $S$-$T_+$ transition via its dependence on $B_{ext}$. This calibration may also be affected by a small measurement-induced polarization, either in the calibration data or at the beginning of each measurement. Finally, the $S$–$T_+$ transition might also shift in response to $\Delta B^z_{nuc}$ rather than just $B_{ext} + B^z_{nuc}$, although we estimate this effect to be negligible at least for values of $\Delta B^z_{nuc} < J(\varepsilon)$.

## IV. LOSS OF CONTRAST FOR LARGE $\Delta B^z_{nuc}$

The data shown in Fig. 2 was taken with the measurement point **M** chosen near the tip of the readout triangle, the region in gate space where spin-blockade can be used for spin to charge conversion. We find that when point **M** is further away from the tip, the amplitude of the observed oscillations decreases with increasing pump time (i.e. oscillation frequency) as show in Supplementary Fig. 3b. For sufficiently large $\Delta B^z_{nuc}$, the oscillations can become entirely invisible. A possible explanation to that could be as follows: if at the measurement point $J < \Delta B^z_{nuc}$, $\Delta B^z_{nuc}$ can drive mixing between $T_0$(1,1) and $S$(1,1). In addition to that, the inelastic relaxation rate between $S$(1,1) and $S$(0,2) can be position dependent. For values of $\varepsilon$ where this relaxation rate is larger than $1/t_M$ ($t_M$ the total measurement time), the triplet $T_0$ can decay within this measurement time and

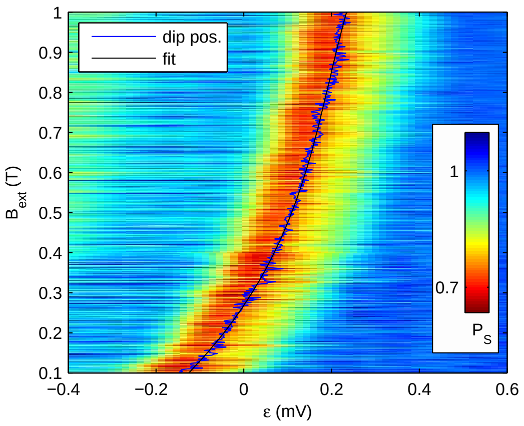


Supplementary Fig. 2: **Calibration of the $S$-$T_+$ transition shift.** Line scans across the $S$-$T_+$ transition vs. $B_{ext}$ used to calibrate the shift of the transition in response to pumping. The $\varepsilon$ axis is given in units of gate voltage and contains an arbitrary offset. The blue line shows the fitted center of the dip in $P_S$ for each scan line and the black line is a polynomial fit to those positions as a function of $B_{ext}$.

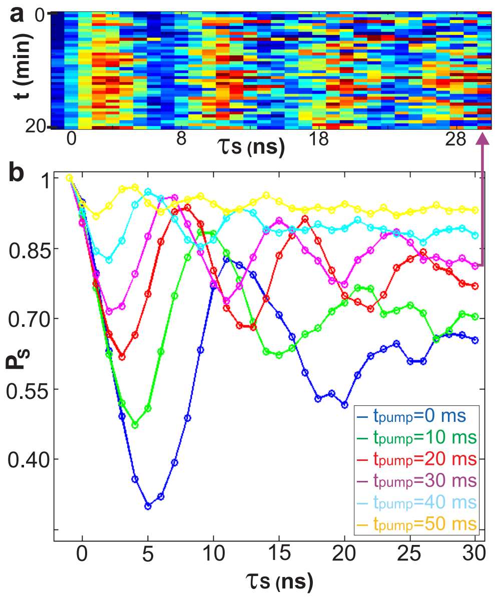


Supplementary Fig. 3: **Contrast loss as a function of polarization. a,** Singlet return probability as a function of separation time $\tau_S$ ($0 \leq \tau_S \leq 30$ ns) for $t_{pump}$=60 ms. **b,** Singlet return probability as a function of $\tau_S$ for different pumping times. The contrast of the signal decreases with increasing pumping time.

spin blockade is lifted. On the other hand if $J \gg \Delta B^z_{nuc}$, mixing does not occur and $T_0$ remains blocked in the (1,1) charge configuration.

By adding an overshoot along the $\varepsilon$ axis (typically by 1.4 mV for 50 ns) when returning from point **S** to point **M**, the contrast can be kept finite even at large $\Delta B^z_{nuc}$. This technique was employed to take the data shown in Fig. 3b. Changes in the pulse distortions due to the setup's finite bandwidth for separation times $\tau_S$ on the order of 100 ns or longer also appear to recover the readout contrast. Presumably, the pulse shape changes in such a way that regions where a large $\Delta B^z_{nuc}$ significantly enhances relaxation are avoided during the readout stage of the pulse. Improvements in the high frequency setup should allow us to understand and/or eliminate these effects. While the above explanations for the contrast loss and recovery are qualitatively consistent with all our data, more work is required to establish their correctness beyond reasonable doubt. However, we are confident that this puzzle does not affect the interpretation of our data in terms of ability to control and utilize $\Delta B^z_{nuc}$ for universal qubit rotations.

## V. MEASUREMENT INDUCED POLARIZATION

Under certain tuning conditions (i.e. specific coupling strengths to the reservoir and between the dots) and certain ranges of magnetic field values, we observe oscillations ($S$–$T_0$ mixing) even without pumping. They appear to be induced by the measurement cycle. Applying $T_+$-pumping monotonically increases their frequency, whereas the $S$-pumping cycle first reduces it until the oscillations disappear. For $S$-pumping with even larger $t_{pump}$, oscillations with increasing frequency reappear. This "spontaneous" $\Delta B^z_{nuc}$ vanishes gradually below $B_{ext} \approx 0.2$ T and typically reaches its maximal value around 0.5 T. At larger fields, it usually decreases but remains substantial up to 1.5 T. Furthermore, it tends to increase when using pulses with overshoots as described in Sec. IV or near the tip of the readout triangle. Various observations suggest that the origin of this polarization is an inelastic decay of triplets at the measurement point, but understanding the details of the unintentional polarization will require further experiments that go beyond the scope of the present work. Since we have demonstrated that intentional pumping can increase or compensate and overcome the measurement induced $\Delta B^z_{nuc}$, it is clear that its presence does not impede the use of dynamic nuclear polarization to achieve quantum control for double quantum dot spin qubits. It is not clear to what extent the polarization effects of the measurement and pump pulses are related, however the fact that $S$-pumping can cancel or overcome the effect of the measurement pulses suggests that the two mechanisms are simply additive.

## VI. TUNING DEPENDENCE

Reilly *et al.* [5] reported a saturation of the mean hyperfine field $B^z_{nuc}$ under $S$-pumping at $B_{ext} + B^z_{nuc} \approx$ 20 mT, whereas we find that a shift of the $S$-$T_+$ transition corresponding to more than 100 mT can be induced

at fields as large as 0.7 T. This discrepancy is at least partly due to the different tuning (i.e. different coupling strength to the reservoir and between the dots) used in the two experiments. Especially the tunnel coupling between the two dots seems to have a considerable influence. As a guide for establishing suitable tuning conditions, we typically measure the current through the double dot as a function of GL and GR for a bias voltage of 0.4 mV across the dot in the non-Pauli blocking direction. Data that is representative for the tuning typically used in the present work is shown in Supplementary Fig. 4a. In Ref. 4, the transport current was typically an order of magnitude smaller [6], similar to our data shown in Supplementary Fig. 4b. A fading signal of the $S$-$T_+$ mixing when increasing the external magnetic field indicates that the transition rate as well as the pumping efficiency are decreasing. For dot tuning shown in Supplementary Fig. 4a, the contrast stays constant at least up to 1.5 T.

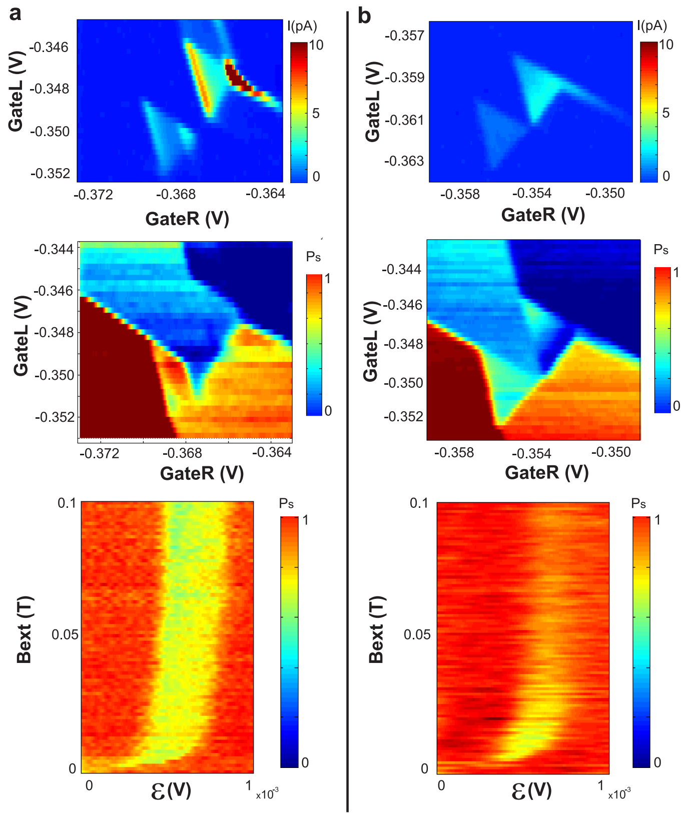


Supplementary Fig. 4: **Two different tuning conditions.** **a,** Current through the dot (upper panel), QPC signal (middle panel) and position of the $S$–$T_+$ transition as a function of magnetic field (lower panel). $\varepsilon$ is given in units of gate voltage with an arbitrary offset). **b,** The same kind of data for tuning conditions more similar to those used in Ref. 4.

[1] A. C. Johnson, J. R. Petta, J. M. Taylor, A. Yacoby, M. D. Lukin, C. M. Marcus, M. P. Hanson, and A. C. Gossard, Nature **435**, 925 (2005).

[2] J. R. Petta, A. C. Johnson, J. M. Taylor, E. A. Laird, A. Yacoby, M. D. Lukin, C. M. Marcus, M. P. Hanson, and A. C. Gossard, Science **309**, 2180 (2005).

[3] E. A. Laird, J. R. Petta, A. C. Johnson, C. M. Marcus, A. Yacoby, M. P. Hanson, and A. C. Gossard, Phys. Rev. Lett. **97**, 056801 (2006).

[4] D. J. Reilly, J. M. Taylor, J. Petta, C. M. Marcus, M. P. Hanson, and A. C. Gossard, Science **321**, 817 (2008).

[5] D. J. Reilly, J. M. Taylor, J. Petta, C. M. Marcus, M. P. Hanson, and A. C. Gossard, *Exchange control of nuclear spin diffusion in double quantum dots* (2008), arXiv:0803.3082v1.

[6] D. J. Reilly, *Private communication.*
